# Supplementary material for: A short note on the computation of the generalised Jacobsthal function for paired progressions
Source: arXiv:1706.03668 ancillary file (2017-06-12)
Supplement: Supplementary file 1 [file full_details.pdf]

# On the computation of the generalised Jacobsthal function for paired progressions

Mario Ziller and John F. Morack

## Abstract

Jacobsthal's function was recently generalised for the case of paired progressions. It was proven that a specific bound of this function is sufficient for the truth of Goldbach's conjecture and of the prime pairs conjecture as well. We review several algorithmic ideas for the computation of the paired Jacobsthal function for primorial numbers and discuss their practicability regarding computational effort. The respective function values were computed for primes up to 73. All these values fulfil the conjectured specific bound. In addition to the results including previously unknown data, we provide exhaustive lists of all sequences of the appropriate maximum lengths in ancillary files.

## 1 Introduction

Henceforth, we denote the set of integral numbers by  $\mathbb{Z}$  and the set of natural numbers, i.e. positive integers, by  $\mathbb{N}$ .  $\mathbb{P} = \{p_i \mid i \in \mathbb{N}\}$  is the set of prime numbers with  $p_1 = 2$ . As usual, we define the  $n^{\text{th}}$  primorial number as the product of the first  $n$  primes:  $p_n\# = \prod_{i=1}^n p_i$ ,  $n \in \mathbb{N}$ . For similar objects of the specific context, we follow the notation of a recent paper [16].

The well known Jacobsthal function [4, 2] was recently generalised for the case of paired progressions [17]. It was proven that a specific upper bound of this function is sufficient for the truth of Goldbach's conjecture and of the prime pairs conjecture as well [17]. In this paper, we will discuss algorithmic approaches for the calculation of the paired Jacobsthal function and present computational results. These approaches were always successfully applied for the computation of the ordinary Jacobsthal function [16]. This paper widely follows the structure of our former paper [16].

In the introduction, we investigate the set of pairs of integers  $\mathbb{Z}^2 = \mathbb{Z} \times \mathbb{Z}$  and first recall some peculiarities of the divisibility of pairs with weak postulations [17]. Afterwards, Jacobsthal's function [4, 2] will be generalised for the case of progressions of consecutive integer pairs using this concept of divisibility [17]. We furthermore define various deduced functions and derive properties which facilitate an effective computation of the appropriate function values.

## Divisibility of integer pairs

**Definition 1.1.** *Divisor of a pair.*

An integer  $k \in \mathbb{Z}$  is a divisor of a pair  $(a, b) \in \mathbb{Z}^2$  if  $k \mid a$  or  $k \mid b$ . We simply write  $k \mid (a, b)$ .

**Remark 1.1.**  $k \mid (a, b) \Rightarrow k \mid a \cdot b$ .

We remark that  $k \mid a \cdot b$  does not necessarily mean  $k \mid (a, b)$ . If  $k = k_1 \cdot k_2$ ,  $k_1 \mid a$ , and  $k_2 \mid b$  then  $k_1 \nmid b$  and  $k_2 \nmid a$  may pertain.

But prime numbers, on the other hand, may be characterised by this condition:

$$p \in \mathbb{P} \Leftrightarrow p \mid a \cdot b \Rightarrow p \mid (a, b).$$

As a consequence of the last definition we declare coprimeness accordingly.

**Definition 1.2.** *Coprime.*

An integer  $k \in \mathbb{Z}$  and a pair  $(a, b) \in \mathbb{Z}^2$  are coprime, and we write  $k \perp (a, b)$ , if  $k \perp a$  and  $k \perp b$ .

**Remark 1.2.**  $k \perp (a, b) \Rightarrow k \nmid a \cdot b$ .

As a conclusion, an integer  $k \in \mathbb{Z}$  and a pair  $(a, b) \in \mathbb{Z}^2$  are not coprime, and we write  $k \not\perp (a, b)$ , if  $k \nmid a$  or  $k \nmid b$ . In other words, there exists an  $k^* \in \mathbb{Z}$  with  $k^* \mid k$  and  $k^* \mid (a, b)$ . Again,  $k$  itself is not necessarily a divisor of  $(a, b)$  here.

## Jacobsthal function

The ordinary Jacobsthal function  $j(n)$  is known to be the smallest natural number  $m$ , such that every sequence of  $m$  consecutive integers contains at least one integer coprime to  $n$  [4, 2].

**Definition 1.3.** *Jacobsthal function.*

For  $n \in \mathbb{N}$ , the Jacobsthal function  $j(n)$  is defined as

$$j(n) = \min \{m \in \mathbb{N} \mid \forall a \in \mathbb{Z} \exists q \in \{1, \dots, m\} : a + q \perp n\}.$$

**Remark 1.3.** This definition is equivalent to the formulation that  $j(n)$  is the greatest difference  $m$  between two terms in the sequence of integers which are coprime to  $n$ .

$$j(n) = \max \{m \in \mathbb{N} \mid \exists a \in \mathbb{Z} : a \perp n \wedge a + m \perp n \wedge \\ \forall q \in \{1, \dots, m-1\} : a + q \not\perp n\}.$$

In other words,  $(j(n) - 1)$  is the greatest length  $m^* = m - 1$  of a sequence of consecutive integers which are not coprime to  $n$ .

An analogous function will be defined below for sequences of integer pairs in place of consecutive integers.

## Paired progressions

Progressions of consecutive pairs in  $\mathbb{Z}^2$  can be defined in an intuitive way. There is a natural duality between a progression of consecutive pairs of integers and a pair of progressions of consecutive integers.

**Definition 1.4.** *Consecutive pairs.*

$(a_1, b_1), (a_2, b_2) \in \mathbb{Z}^2$  are called consecutive pairs if  $a_2 = a_1 + 1$  and  $b_2 = b_1 + 1$ .  $(a_2, b_2)$  is called successor of  $(a_1, b_1)$ .

**Definition 1.5.** *Paired progression.*

An ordered sequence of consecutive pairs  $\{(a_i, b_i) \in \mathbb{Z}^2\}_{i=1, \dots, k}$  is called a paired progression if  $(a_{i+1}, b_{i+1})$  is a successor of  $(a_i, b_i)$  for  $i = 1, \dots, k-1$ .

**Remark 1.4.** For every paired progression  $\{(a_i, b_i) \in \mathbb{Z}^2\}_{i=1, \dots, k}$  as defined above, there exists a pair  $(a, b) \in \mathbb{Z}^2$  with  $(a_i, b_i) = (a + i, b + i)$  for  $i = 1, \dots, k$ . We use the notation  $\langle a, b \rangle_k$  for this paired progression and point to the fact that  $(a, b)$  itself is not member of the progression.

## Generalised Jacobsthal function

We now generalise Jacobsthal's function on successive pairs of integers as its canonical extension to paired progressions and apply weak divisibility at it.

**Definition 1.6.** *Paired Jacobsthal function.*

Let  $n$  be a natural number. The paired Jacobsthal function  $j_2(n)$  is defined to be the smallest natural number  $m$ , such that every paired progression  $\langle a, b \rangle_m$  of length  $m$  with an even difference of its pair elements contains at least one pair coprime to  $n$ .

$$\begin{aligned} j_2(n) &= \min \{m \in \mathbb{N} \mid \forall (a, b) \in \mathbb{Z}^2 \text{ with } 2 \mid (b - a) : \\ &\quad \exists (x, y) \in \langle a, b \rangle_m : n \perp (x, y)\}, \\ \text{or } j_2(n) &= \min \{m \in \mathbb{N} \mid \forall (a, b) \in \mathbb{Z}^2 \text{ with } 2 \mid (b - a) : \\ &\quad \exists q \in \{1, \dots, m\} : n \perp (a + q, b + q)\}. \end{aligned}$$

**Remark 1.5.** In the particular case of an odd difference of the pair elements, there is no pair coprime to an even  $n$  because either the first or the second element of the pair would be even. This trivial case must be excluded. Otherwise  $j_2(n)$  would not be defined for even  $n$ .

This definition is equivalent to the formulation that the paired Jacobsthal function  $j_2(n)$  is the greatest difference  $m$  between two pairs in a sequence of consecutive pairs with an even difference of its pair elements, which are coprime to  $n$ .

$$\begin{aligned} j_2(n) &= \max \{m \in \mathbb{N} \mid \exists (a, b) \in \mathbb{Z}^2 \text{ with } 2 \mid (b - a) : \\ &\quad n \perp (a, b) \wedge n \perp (a + m, b + m) \wedge \\ &\quad \forall q \in \{1, \dots, m-1\} : n \not\perp (a + q, b + q)\}. \end{aligned}$$

In other words,  $(j_2(n) - 1)$  is the greatest length  $m^* = m - 1$  of a paired progression  $\langle a, b \rangle_{m^*}$  with an even difference of its pair elements where no pair is coprime to  $n$ . For this reason, we define a reduced variant of the paired Jacobsthal function. This will make a simplified representation possible.

**Definition 1.7.** *Reduced paired Jacobsthal function.*

For  $n \in \mathbb{N}$ , the reduced paired Jacobsthal function  $j_2^*(n)$  is defined as

$$\begin{aligned} j_2^*(n) &= j_2(n) - 1, \\ j_2^*(n) &= \max \{m^* \in \mathbb{N} \mid \exists (a, b) \in \mathbb{Z}^2 \text{ with } 2 \mid (b - a) : \\ &\quad \forall q \in \{1, \dots, m^*\} : n \nmid (a + q, b + q)\}. \end{aligned}$$

**Remark 1.6.** The following statements are elementary consequences of the definition 1.6 of the paired Jacobsthal function and describe some interesting properties of it. Equivalent properties are known for the common Jacobsthal function for integer sequences [4, 16].

Product.

$$\forall n_1, n_2 \in \mathbb{N} : j_2(n_1 \cdot n_2) \geq j_2(n_1) \wedge j_2(n_1 \cdot n_2) \geq j_2(n_2).$$

Coprime product.

$$\forall n_1, n_2 \in \mathbb{N} > 1 \mid n_1 \perp n_2 : j_2(n_1 \cdot n_2) > j_2(n_1) \wedge j_2(n_1 \cdot n_2) > j_2(n_2).$$

Greatest common divisor.

$$\forall n_1, n_2 \in \mathbb{N} : j_2(\gcd(n_1, n_2)) \leq j_2(n_1) \wedge j_2(\gcd(n_1, n_2)) \leq j_2(n_2).$$

Prime power.

$$\forall n, k \in \mathbb{N} \forall p \in \mathbb{P} : j_2(p^k \cdot n) = j_2(p \cdot n).$$

Prime separation.

$$\forall n, n^*, k \in \mathbb{N} \forall p \in \mathbb{P} \mid n = p^k \cdot n^*, p \perp n^* : j_2(n) = j_2(p \cdot n^*).$$

The last remark implies that the entire paired Jacobsthal function is also determined by its values for products of distinct primes. The particular case of primorial numbers is therefore most interesting because the function values at these points contain the relevant information for constructing general upper bounds. The paired Jacobsthal function of primorial numbers  $h_2(n)$  is therefore defined as the smallest natural number  $m$ , such that every paired progression  $\langle a, b \rangle_m$  of length  $m$  with  $2 \mid (b - a)$  contains at least one pair coprime to the product of the first  $n$  primes.

**Definition 1.8.** *Primorial paired Jacobsthal function.*

For  $n \in \mathbb{N}$ , the primorial paired Jacobsthal function  $h_2(n)$  is defined as

$$h_2(n) = j_2(p_n\#).$$

By analogy with definition 1.7, we also define a reduced variant of the latter function which represents the greatest length of a paired progression  $\langle a, b \rangle_{m^*}$  with  $2 \mid (b - a)$  the elements of which are not coprime to the  $n^{\text{th}}$  primorial number.

**Definition 1.9.** *Reduced primorial paired Jacobsthal function.*

For  $n \in \mathbb{N}$ , the reduced primorial paired Jacobsthal function  $h_2^*(n)$  is defined as

$$\begin{aligned} h_2^*(n) &= h_2(n) - 1, \\ h_2^*(n) &= \max \{m^* \in \mathbb{N} \mid \exists (a, b) \in \mathbb{Z}^2 \text{ with } 2 \mid (b - a) : \\ &\quad \forall q \in \{1, \dots, m^*\} : p_n\# \nmid (a + q, b + q)\}. \end{aligned}$$

By definition,  $h_2^*(n)$  is the greatest length  $m^*$  of a paired progression  $\langle a, b \rangle_{m^*}$  with  $2 \mid (b - a)$  the elements of which are not coprime to the product of the first  $n$  primes. This means that every pair in the progression must be divisible by at least one of these primes.

For the effective computation of  $h_2(n)$ , or  $h_2^*(n)$  respectively, it is sufficient to omit the primes 2 and 3 from the calculation as will be demonstrated below. Therefore, we define a condensed Jacobsthal function  $\omega_2(n)$  which is directly related to  $h_2(n)$ . Its computation reduces unnecessary effort. We harmonise the arguments of the functions  $\omega_2(n)$  and  $h_2(n)$  so that  $n$  in both of them refer to the greatest considered prime  $p_n$  with  $n > 2$ .

**Definition 1.10.** *Condensed paired Jacobsthal function.* [12]

For  $n \in \mathbb{N} > 2$ , the condensed paired Jacobsthal function  $\omega_2(n)$  is defined as the greatest length of a paired progression with an even difference of its pair elements where for every pair at least one of the primes  $p_3$  to  $p_n$  is a divisor.

$$\omega_2(n) = j^*(p_n\#/6).$$

The primes 2 and 3 play a specific role for the paired Jacobsthal function. The following lemmata describe interesting properties of it and make the direct calculation of  $j_2(n)$  as a function of  $\omega_2(n)$  possible.

**Lemma 1.1.** *Let  $n \in \mathbb{N}$  with  $2 \nmid n$ . Then*

$$j_2(2 \cdot n) = 2 \cdot j_2(n).$$

*Proof.* We get  $j_2(1) = 1$  because every natural number is coprime to 1. Furthermore,  $j_2(2) = 2$  because every sequence of two consecutive integers contains one even and one odd number. So, one of every two consecutive integer pairs with even differences of the pair elements contains only odd numbers.

Let now  $n > 1$ . According to definition 1.7, we resume

$$j_2(n) = \max \{m \in \mathbb{N} \mid \exists (a, b) \in \mathbb{Z}^2 \text{ with } 2 \mid (b - a) : \\ \forall q \in \{1, \dots, m - 1\} : n \nmid (a + q, b + q)\}.$$

Given  $m \in \mathbb{N}$  and  $a, b \in \mathbb{Z}$  as above. Then, there exist  $a^*, b^* \in \mathbb{Z}$  with  $a^* \equiv 2 \cdot a \pmod{n}$ ,  $b^* \equiv 2 \cdot b \pmod{n}$ ,  $a^* \equiv 1 \pmod{2}$ , and  $b^* \equiv 1 \pmod{2}$  due to the Chinese remainder theorem. We get  $2 \mid (b^* - a^*)$  because  $a^* \equiv b^* \equiv 1 \pmod{2}$ .

With such  $a^*, b^*$ , we conclude for  $q = 1, \dots, m - 1$

$$\begin{aligned} a^* + 2 \cdot q &\equiv 2 \cdot a + 2 \cdot q \equiv 2 \cdot (a + q) \pmod{n}, \\ b^* + 2 \cdot q &\equiv 2 \cdot b + 2 \cdot q \equiv 2 \cdot (b + q) \pmod{n}, \\ a^* + 2 \cdot q - 1 &\equiv 1 + 2 \cdot q - 1 \equiv 0 \pmod{2}, \text{ and} \\ b^* + 2 \cdot q - 1 &\equiv 1 + 2 \cdot q - 1 \equiv 0 \pmod{2}. \end{aligned}$$

Because in addition  $a^* + 2 \cdot m - 1 \equiv 0 \pmod{2}$  and  $b^* + 2 \cdot m - 1 \equiv 0 \pmod{2}$ ,

$$\exists (a^*, b^*) \in \mathbb{Z}^2 \text{ with } 2 \mid (b^* - a^*) : \forall q \in \{1, \dots, 2 \cdot m - 1\} : 2 \cdot n \nmid (a^* + q, b^* + q)\}$$

holds, and  $j_2(2 \cdot n) \geq 2 \cdot m = 2 \cdot j_2(n)$  follows. The maximality remains retained in both directions.  $\square$

**Lemma 1.2.** *Let  $n \in \mathbb{N}$  with  $3 \nmid n$ . Then*

$$j_2(3 \cdot n) = 3 \cdot j_2(n).$$

*Proof.* We recall  $j_2(1) = 1$  and get  $j_2(3) = 3$  because 3 is not coprime to both pairs of  $\langle 2, 4 \rangle_2$ . Considering however all possible remainder combinations modulo 3, 3 is coprime to at least one of every three consecutive integer pairs with even differences of the pair elements.

Let now  $n > 1$ . Given  $m = j_2^*(n)$ ,  $a, b \in \mathbb{Z}$  with  $2 \mid (b - a)$ , and

$$\forall q \in \{1, \dots, m - 1\} : n \nmid (a + q, b + q).$$

According to the Chinese remainder theorem, there exist  $a^*, b^* \in \mathbb{Z}$  with  $a^* \equiv 3 \cdot a \pmod{n}$ ,  $b^* \equiv 3 \cdot b \pmod{n}$ ,  $a^* \equiv 1 \pmod{3}$ , and  $b^* \equiv 2 \pmod{3}$ , and in addition  $a^* \equiv 3 \cdot a \pmod{2}$ ,  $b^* \equiv 3 \cdot b \pmod{2}$  if  $2 \nmid n$ .

We get  $b^* - a^* \equiv 3 \cdot a - 3 \cdot b = 3 \cdot (b - a) \equiv 0 \pmod{2}$ .

With such  $a^*, b^*$ , we conclude for  $q = 1, \dots, m - 1$

$$\begin{aligned} a^* + 3 \cdot q &\equiv 3 \cdot a + 3 \cdot q \equiv 3 \cdot (a + q) \pmod{n}, \\ b^* + 3 \cdot q &\equiv 3 \cdot b + 3 \cdot q \equiv 3 \cdot (b + q) \pmod{n}, \\ a^* + 3 \cdot q - 1 &\equiv 1 + 3 \cdot q - 1 \equiv 0 \pmod{3}, \text{ and} \\ b^* + 3 \cdot q - 2 &\equiv 2 + 3 \cdot q - 2 \equiv 0 \pmod{3}. \end{aligned}$$

Because in addition  $a^* + 3 \cdot m - 1 \equiv 0 \pmod{3}$  and  $b^* + 3 \cdot m - 2 \equiv 0 \pmod{3}$ ,

$$\exists (a^*, b^*) \in \mathbb{Z}^2 \text{ with } 2 \mid (b^* - a^*) : \forall q \in \{1, \dots, 3 \cdot m - 1\} : 3 \cdot n \nmid (a^* + q, b^* + q)$$

holds, and  $j_2(3 \cdot n) \geq 3 \cdot m = 3 \cdot j_2(n)$  follows. The maximality remains retained in both directions.  $\square$

**Corollary 1.3.** *Let  $n \in \mathbb{N} > 2$ .*

$$h_2(n) = 6 \cdot \omega_2(n) + 6.$$

*Proof.*

$$\begin{aligned} j_2(3 \cdot p_n\#/6) &= j_2(p_n\#/2) = 3 \cdot j_2(p_n\#/6) \\ j_2(2 \cdot p_n\#/2) &= j_2(p_n\#) = 2 \cdot j_2(p_n\#/2) \\ \omega_2(n) &= j_2^*(p_n\#/6) = j_2(p_n\#/6) - 1 = j_2(p_n\#)/6 - 1. \\ h_2(n) &= j_2(p_n\#) = 6 \cdot \omega_2(n) + 6. \end{aligned}$$

$\square$

The function  $\omega_2(n)$  is only defined for  $n > 2$ . For  $n \leq 2$ , we get  $h_2(1) = j_2(2) = 2$  and  $h_2(2) = j_2(6) = 3 \cdot j_2(2) = 6$ .

The counting of  $\omega_2(n)$  remains the central computational problem. By definition,  $\omega_2(n)$  is the greatest length of a paired progression with an even difference of its pair elements where no pair is coprime to all of the  $n - 2$  primes  $p_3, \dots, p_n$ . This means that for every pair at least one of the primes  $p_3$  to  $p_n$  must be a divisor.

The definition of  $\omega_2(n)$  can be extended to all paired progressions. The demand for an even difference of the pair elements is not necessary any more because only odd primes must be considered.

**Lemma 1.4.** For every paired progression  $\langle a, b \rangle_m$  with  $2 \mid (b - a)$ , there exists a paired progression  $\langle a, b^* \rangle_m$  with  $2 \nmid (b^* - a)$ , and vice versa, so that both progressions have the same divisibility characteristics for the primes  $p_3, \dots, p_n$ .

*Proof.* In consequence of the Chinese remainder theorem, there exists  $b^* \in \mathbb{Z}$  with  $b^* \equiv b + 1 \pmod{2}$  and  $b^* \equiv b \pmod{p_i}$  for  $i = 3, \dots, n$ . Thus  $2 \mid (b - a)$  if and only if  $2 \nmid (b^* - a)$ . On the other hand, we have  $p_i \mid (a + q, b + q)$  if and only if  $p_i \mid (a + q, b^* + q)$  for all  $i = 3, \dots, n$  and all  $q = 1, \dots, m$ .  $\square$

Paired progressions where each of the primes  $p_3$  to  $p_n$  is a divisor of at least one of its pairs can otherwise be characterised by a choice of two non-zero residue classes for each prime, or alternatively by a permutation of the set  $\{p_3, \dots, p_n\}$  with two repetitions each element where the sequence is filled from left to right covering the next free position each time recursively.

**Proposition 1.5.** Let  $m, n \in \mathbb{N}$ ,  $n > 2$ .

The following three statements are equivalent if  $m = \omega_2(n)$ .

- (1) There exists a pair  $(a, b) \in \mathbb{Z}^2$  so that for every element of the paired progression  $\langle a, b \rangle_m$  one of the primes  $p_3, \dots, p_n$  is a divisor.

$$\exists (a, b) \in \mathbb{Z}^2 \forall q \in \{1, \dots, m\} \exists i \in \{3, \dots, n\} : a + q \equiv 0 \vee b + q \equiv 0 \pmod{p_i}.$$

- (2) For every prime  $p_3, \dots, p_n$ , there exist two non-zero residue classes so that every integer of the sequence  $\{1, \dots, m\}$  belongs to one of them.

$$\begin{aligned} &\exists a_i, b_i \in \{1, \dots, p_i - 1\}, i = 3, \dots, n : \\ &\forall q \in \{1, \dots, m\} \exists i \in \{3, \dots, n\} : q \equiv a_i \vee q \equiv b_i \pmod{p_i}. \end{aligned}$$

- (3) There exists a permutation  $(\pi_1, \dots, \pi_{2n-4})$  of  $\{p_3, \dots, p_n\}$  with twofold repetition and a tuple  $(q_1, \dots, q_{2n-4})$  so that the sequence  $\{1, \dots, m\}$  is completely covered by the residue classes  $q_i \pmod{\pi_i}$  when all  $\pi_i$  were recursively assigned to the first free position  $q_i$ , respectively.

$$\begin{aligned} &\exists \pi_i \in \{p_3, \dots, p_n\} \exists q_i \in \{1, \dots, m\}, i = 1, \dots, 2n - 4 \\ &\text{with } (\{\pi_1, \dots, \pi_{2n-4}\} \setminus \{p_3, \dots, p_n\}) \setminus \{p_3, \dots, p_n\} = \emptyset, \\ &q_i \not\equiv 0 \pmod{\pi_i}, i = 1, \dots, 2n - 4, \\ &i < j \Rightarrow q_i < q_j, i, j \in \{1, \dots, 2n - 4\}, \\ &q_1 = 1, \text{ and} \\ &q_i = \min\{j \in \{1, \dots, m\} \mid \forall k < i : j \not\equiv q_k \pmod{\pi_k}\}, i = 2, \dots, 2n - 4 : \\ &\forall q \in \{1, \dots, m\} \exists i \in \{1, \dots, 2n - 4\} : q \equiv q_i \pmod{\pi_i}. \end{aligned}$$

*Proof.*

(1)  $\Rightarrow$  (2):

$a_i \equiv -a, b_i \equiv -b \pmod{p_i}, i = 3, \dots, n$  satisfy the respective congruences of (2).  $p_i \nmid a$  and  $p_i \nmid b$  because  $m$  is maximum.

(2)  $\Rightarrow$  (3):

We set  $q_1 = 1$  and choose  $\pi_1$  as the smallest  $p_j$  with  $a_j \equiv q_1$  or  $b_j \equiv q_1 \pmod{p_j}$ . Given  $q_k$  and  $\pi_k$  for  $1 \leq k < i \leq 2n - 4$ , we set  $q_i = \min\{j \in \{1, \dots, m\} \mid \forall k < i : j \not\equiv q_k \pmod{\pi_k}\}$ . Then we choose  $\pi_i$  as the smallest  $p_j$  with  $a_j \equiv q_i$  or  $b_j \equiv q_i \pmod{p_j}$ . There must exist a proper  $p_j$  because  $m = \omega_2(n)$ . Otherwise, at least  $p_j$  was not needed two times to cover a sequence of length  $m$  and this sequence could be extended to a longer one by setting  $q_i = m + 1$  and  $\pi_i = p_j$  which contradicts to the definition of  $\omega_2(n)$ . All  $q_i$  and  $\pi_i$  inductively selected as described above fulfils (3).

(3)  $\Rightarrow$  (1):

For every  $i \in \{3, \dots, n\}$ , there exist two indices  $j_a, j_b \in \{1, \dots, 2n - 4\}$  with  $\pi_{j_a} = \pi_{j_b} = p_i$  because  $(\pi_1, \dots, \pi_{2n-4})$  is a permutation of  $\{p_3, \dots, p_n\}$  with twofold repetition.

According to the Chinese remainder theorem, there exist  $a, b \in \mathbb{Z}$  solving the systems of simultaneous congruences  $a \equiv -q_{j_a}$  and  $b \equiv -q_{j_b} \pmod{p_i}$ ,  $i = 3, \dots, n$ . The solutions  $a$  and  $b$  fulfil (1).  $\square$

**Remark 1.7.** If  $p_i \nmid a$  and  $p_i \nmid b$  were required for all  $i = 3, \dots, n$  then the proposition holds for the properties (1) and (2) even if  $m < \omega_2(n)$ .

The set of sequences with the property (2) includes any sequence fulfilling (3), even if  $m < \omega_2(n)$ . The maximality of  $m$  was only used in the part (2)  $\Rightarrow$  (3) of the proof.

Furthermore, the proposition holds for any set of distinct primes. The specific choice of the primes was not used in the proof.

**Corollary 1.6.** *For every sequence of maximum length satisfying proposition 1.5 (2), there exists a reverse sequence with*

$$\begin{aligned} &\exists c_i, d_i \in \{1, \dots, p_i - 1\}, i = 3, \dots, n : \\ &\forall q \in \{1, \dots, m\} \exists i \in \{3, \dots, n\} : m + 1 - q \equiv c_i \vee m + 1 - q \equiv d_i \pmod{p_i}. \end{aligned}$$

*Proof.* The maximality of the given sequence length implies  $m + 1 \not\equiv a_i$  and  $m + 1 \not\equiv b_i \pmod{p_i}$  for all  $i = 3, \dots, n$ . Therefore,  $c_i \equiv m + 1 - a_i \pmod{p_i}$  and  $d_i \equiv m + 1 - b_i \pmod{p_i}$  satisfy the requirements for  $i = 3, \dots, n$ .  $\square$

The pairs of reverse sequences define a symmetry within the set of sequences of maximum length. The algorithmic exploitation of this interesting feature, however, seems to be difficult because  $m$  is a priori unknown.

**Example 1.1.** We give an example for  $n = 5$  for all of the three variants of the proposition 1.5. The primes to be considered are 5, 7, and 11. The result  $\omega_2(n)=10$  is reached in a sequence with the following properties:

Prime sequence. Property (1).

$$a = 468, b = 676.$$

$$7/(a + 1), 5/(a + 2), 7/(b + 3), 5/(b + 4), 11/(a + 5),$$

$$11/(b + 6), 5/(a + 7), 7/(a + 8), 5/(b + 9), 7/(b + 10).$$



Set of remainders. Property (2).

$$\begin{aligned} a_3 = 2, b_3 = 4, a_4 = 1, b_4 = 3, a_5 = 5, b_5 = 6. \\ 1 \equiv 1 \pmod{7}, 2 \equiv 2 \pmod{5}, 3 \equiv 3 \pmod{7}, 4 \equiv 4 \pmod{5}, 5 \equiv 5 \pmod{11}, \\ 6 \equiv 6 \pmod{11}, 7 \equiv 2 \pmod{5}, 8 \equiv 1 \pmod{7}, 9 \equiv 4 \pmod{5}, 10 \equiv 3 \pmod{7}. \end{aligned}$$

Prime Permutation. Property (3).

$$\begin{aligned} \pi_1 = 7, \pi_2 = 5, \pi_3 = 7, \pi_4 = 5, \pi_5 = 11, \pi_6 = 11. \\ q_1 = 1, q_2 = 2, q_3 = 3, q_4 = 4, q_5 = 5, q_6 = 6. \\ 1 \equiv 1 \pmod{7}, 2 \equiv 2 \pmod{5}, 3 \equiv 3 \pmod{7}, 4 \equiv 4 \pmod{5}, 5 \equiv 5 \pmod{11}, \\ 6 \equiv 6 \pmod{11}, 7 \equiv 2 \pmod{5}, 8 \equiv 1 \pmod{7}, 9 \equiv 4 \pmod{5}, 10 \equiv 3 \pmod{7}. \end{aligned}$$

**Remark 1.8.** As a consequence of proposition 1.5, we can formulate three equivalent descriptions of the condensed Jacobsthal function  $\omega_2(n)$  for  $n > 2$ .

- (1) The function  $\omega_2(n)$  is the maximum length  $m$  of a paired progression so that for every pair of it one of the primes  $p_3, \dots, p_n$  is a divisor.

$$\begin{aligned} \omega_2(n) = \max \{m \in \mathbb{N} \mid \exists (a, b) \in \mathbb{Z}^2 \\ \forall q \in \{1, \dots, m\} \exists i \in \{3, \dots, n\} : a+q \equiv 0 \vee b+q \equiv 0 \pmod{p_i}\}. \end{aligned}$$

- (2) The function  $\omega_2(n)$  is the maximum  $m \in \mathbb{N}$  for which there exist sets of non-zero remainders  $a_i \pmod{p_i}$  and  $b_i \pmod{p_i}$ ,  $i = 3, \dots, n$  so that every  $q \in \{1, \dots, m\}$  satisfies one of the congruences  $q \equiv a_i$  or  $q \equiv b_i \pmod{p_i}$ .

$$\begin{aligned} \omega_2(n) = \max \{m \in \mathbb{N} \mid \exists a_i, b_i \in \{1, \dots, p_i - 1\}, i = 3, \dots, n : \\ \forall q \in \{1, \dots, m\} \exists i \in \{3, \dots, n\} : q \equiv a_i \vee q \equiv b_i \pmod{p_i}\}. \end{aligned}$$

- (3) The function  $\omega_2(n)$  is the maximum  $m \in \mathbb{N}$  for which there exist a permutation  $(\pi_1, \dots, \pi_{2n-4})$  of  $\{p_3, \dots, p_n\}$  with twofold repetition and a tuple  $(q_1, \dots, q_{2n-4})$  so that the sequence  $\{1, \dots, m\}$  is completely covered by the residue classes  $q_i \pmod{\pi_i}$  when all  $\pi_i$  were recursively assigned to the first free position  $q_i$ , respectively.

$$\begin{aligned} \omega_2(n) = \max \{m \in \mathbb{N} \mid \exists \pi_i \in \{p_3, \dots, p_n\} \exists q_i \in \{1, \dots, m\}, i = 1, \dots, 2n-4 \\ \text{with } (\{\pi_1, \dots, \pi_{2n-4}\} \setminus \{p_3, \dots, p_n\}) \setminus \{p_3, \dots, p_n\} = \emptyset, \\ q_i \not\equiv 0 \pmod{\pi_i}, i = 1, \dots, 2n-4, \\ i < j \Rightarrow q_i < q_j, i, j \in \{1, \dots, 2n-4\}, \\ q_1 = 1, \text{ and for } i = 2, \dots, 2n-4 \\ q_i = \min\{j \in \{1, \dots, m\} \mid \forall k < i : j \not\equiv q_k \pmod{\pi_k}\} : \\ \forall q \in \{1, \dots, m\} \exists i \in \{1, \dots, 2n-4\} : q \equiv q_i \pmod{\pi_i}\}. \end{aligned}$$

In the next chapter, we will recall several algorithmic ideas for the computation of the paired Jacobsthal function for primorial numbers which were successfully applied to the conventional Jacobsthal function for primorials [16]. All of these approaches utilise the versions (2) or (3) of understanding  $\omega_2(n)$ . When we present our results below, we will get back to the recent remark in order to derive demonstrative forms for the presentation of sequences.

## 2 Computation of $\omega_2(n)$

Several approaches were described for the computation of Jacobsthal's function for primorials [16]. We recall these algorithmic ideas and adapt them for their application to the extended, paired Jacobsthal function for primorials. The number '2' was added to the names of the algorithms to avoid confusion.

### 2.1 Basic algorithms

Brute force is the most obvious idea for computing  $\omega_2(n)$ . All possible remainder combinations according to proposition 1.5, statement (2), are processed sequentially. To each of them, a fill&cont procedure is applied as follows. For each of the residue classes, all positions of a previously empty array of sufficient length covered by that residue class are labelled. The first unlabelled position corresponds to  $m + 1$  where  $m$  is the length of the related sequence. This length is then registered for searching the maximum possible length.

This naïve algorithm is henceforth referred to as Basic Sequential Algorithm 2 (BSA2). It can be implemented as a recursive procedure as depicted in the pseudocode 1.

---

**Algorithm 1** Basic Sequential Algorithm 2 (BSA2).

---

```

procedure BASIC_SEQUENTIAL_2(arr,k)
  for i=1 to plist[k]-2 do
    arr1=arr; fill_array(arr1,i,plist[k])
    for j=i+1 to plist[k]-1 do
      arr2=arr1; fill_array(arr2,j,plist[k])
      if k<n-2 then basic_sequential_2(arr2,k+1)
      else count_array(arr2)
      end if
    end for
  end for
end procedure
arr=empty_array
plist=[ $p_3, \dots, p_n$ ]
k=1
basic_sequential_2(arr,k)

```

▷ Sequence array  
 ▷ Array of primes  
 ▷ Starting prime array index  
 ▷ Recursion

---

The filling of a previously empty array of sufficient length from left to right according to proposition 1.5, statement (3), is another simple idea for computing  $\omega_2(n)$ . All permutations  $(\pi_1, \dots, \pi_{2n-4})$  of the given primes  $\{p_3, \dots, p_n\}$  with twofold repetition are processed sequentially. Starting with position 1, the first prime  $\pi_1$  is chosen and with it the residue class  $1 \bmod \pi_1$ . After labelling all positions covered by that residue class, the next unlabelled position is searched and the next prime of the permutation under consideration is analogously used until all primes are consumed.

If in any case a prime divides the index of the next unlabelled position then this case can be omitted because only non-zero residue classes are appropriate. Handling all permutations where primes are not divisors of their related position-numbers will therefore discover all sequences of the maximum possible length. An additional counter was incorporated for every prime to distinguish whether one or two instances of the regarded prime are left untreated in the permutation. The Basic Permutation Algorithm 2 is described in pseudocode 2.

---

**Algorithm 2** Basic Permutation Algorithm 2 (BPA2).

---

```

procedure BASIC_PERMUTATION_2(arr,plist,clist,k,q)
  for i=k to n-2 do
    if  $q \not\equiv 0 \pmod{\text{plist}[i]}$  then
      arr1=arr; fill_array(arr1,q,plist[i])
      q1=next_free_position(arr1)
      plist1=plist; clist1=clist
      if clist[i]=2 then
        clist1[i]=1
        k1=k
        basic_permutation_2(arr1,plist1,clist1,k1,q1)
      else
        if k<n-2 then
          interchange(plist1[k],plist1[i])
          interchange(clist1[k],clist1[i])
          k1=k+1
          basic_permutation_2(arr1,plist1,clist1,k1,q1)
        else count_array(arr1)
      end if
    end if
  end for
end procedure
arr=empty_array
plist=[ $p_3, \dots, p_n$ ]
clist=[2,...,2]
k=1
q=1
basic_permutation_2(arr,plist,clist,k,q)

```

- ▷ Sequence array
  - ▷ Array of primes
  - ▷ Array of prime counters
  - ▷ Starting prime array index
  - ▷ Starting sequence position
  - ▷ Recursion
-

Both of the presented algorithms are not really effective for practical purpose. A simple estimation of their complexities reveals the problem. The number  $N_{BSA2}$  of residue class combinations in the Basic Sequential Algorithm 2 is

$$N_{BSA2} = \prod_{i=3}^n \frac{(p_i - 1) \cdot (p_i - 2)}{2}.$$

For the Basic Permutation Algorithm 2, we have

$$N_{BPA2} \leq \frac{(2 \cdot n - 4)!}{2^{n-2}} \ll N_{BSA2}.$$

However,  $\frac{(2n-4)!}{2^{n-2}}$  also grows too fast to be reasonable. In the upcoming sections, we describe possibilities of how to dramatically reduce the number of sequences which are needed to be considered for determining  $\omega_2(n)$ .

The Basic Permutation Algorithm 2 as described above is ineffective for another reason. There may exist different, equivalent permutations constituting the same sequence. In this case, only one of these permutations must be examined. Selecting the smallest prime if there are any at choice, defines the additional rule of a Reduced Permutation Algorithm 2 (RPA2) [13] which thereby also downsizes the number of permutations needed to be considered. This principle was yet applied in part (2)  $\Rightarrow$  (3) of the proof of proposition 1.5. The Basic Permutation Algorithm 2 indeed produces doublets of sequences.

**Proposition 2.1.** *Let  $m, n \in \mathbb{N}$ ,  $n > 2$ , and  $m = \omega_2(n)$ .*

*Given a permutation  $(\pi_1, \dots, \pi_{2n-4})$  of  $\{p_3, \dots, p_n\}$  with twofold repetition and a tuple  $(q_1, \dots, q_{2n-4})$  so that the sequence  $\{1, \dots, m\}$  is completely covered by the residue classes  $q_i \bmod \pi_i$  when all  $\pi_i$  were recursively assigned to the first free position  $q_i$ , respectively. And let  $q_{k_1} \equiv q_{k_2} \pmod{\pi_{k_2}}$ ,  $k_1 < k_2$ , for any  $k_1, k_2 \in \{1, \dots, 2n-4\}$ .*

$$\begin{aligned} &\forall q \in \{1, \dots, m\} \exists i \in \{1, \dots, 2n-4\} : q \equiv q_i \pmod{\pi_i} \\ &\text{where } \pi_i \in \{p_3, \dots, p_n\}, q_i \in \{1, \dots, m\}, i = 1, \dots, 2n-4, \\ &(\{\pi_1, \dots, \pi_{2n-4}\} \setminus \{p_3, \dots, p_n\}) \setminus \{p_3, \dots, p_n\} = \emptyset, \\ &q_i \not\equiv 0 \pmod{\pi_i}, i = 1, \dots, 2n-4, \\ &i < j \Rightarrow q_i < q_j, i, j \in \{1, \dots, 2n-4\}, \\ &q_1 = 1, \text{ and} \\ &q_i = \min\{j \in \{1, \dots, m\} \mid \forall k < i : j \not\equiv q_k \pmod{\pi_k}\}, i = 2, \dots, 2n-4, \\ &\text{and} \\ &\exists k_1, k_2 \in \{1, \dots, 2n-4\}, k_1 < k_2 : q_{k_1} \equiv q_{k_2} \pmod{\pi_{k_2}}. \end{aligned}$$

*Then there exist an equivalent permutation  $(\varrho_1, \dots, \varrho_{2n-4})$  of  $\{p_3, \dots, p_n\}$  with twofold repetition and a tuple  $(r_1, \dots, r_{2n-4})$  according to proposition 1.5, statement (3) so that  $\varrho_k = \pi_k$ ,  $r_k = q_k$  for  $k < k_1$  if exist, and  $\varrho_{k_1} = \pi_{k_2}$ ,  $r_{k_1} = q_{k_1}$ . Furthermore for  $k > k_1$  if exist,  $r_k \equiv q_j \pmod{\varrho_k}$  if  $\varrho_k = \pi_j$ .*

$\exists q_i \in \{p_3, \dots, p_n\} \exists r_i \in \{1, \dots, m\}, i = 1, \dots, 2n - 4$   
*with*  $(\{q_1, \dots, q_{2n-4}\} \setminus \{p_3, \dots, p_n\}) \setminus \{p_3, \dots, p_n\} = \emptyset,$   
 $r_i \not\equiv 0 \pmod{q_i}, i = 1, \dots, 2n - 4,$   
 $i < j \Rightarrow r_i < r_j, i, j \in \{1, \dots, 2n - 4\},$   
 $r_1 = 1,$   
 $r_i = \min\{j \in \{1, \dots, m\} \mid \forall k < i : j \not\equiv r_k \pmod{q_k}\}, i = 2, \dots, 2n - 4,$   
 $\forall q \in \{1, \dots, m\} \exists i \in \{1, \dots, 2n - 4\} : q \equiv r_i \pmod{q_i},$   
*so that*  
 $\forall k \in \{1, \dots, 2n - 4\}, k < k_1 : q_k = \pi_k \wedge r_k = q_k,$   
 $q_{k_1} = \pi_{k_2}, r_{k_1} = q_{k_1},$  *and*  
 $\forall k \in \{1, \dots, 2n - 4\}, k > k_1 : r_k \equiv q_j \pmod{q_k} \text{ if } q_k = \pi_j.$

*Proof.* According to the assumptions,  $r_i$  and  $q_i$  satisfy the requirements for  $i \leq k_1$ . Given  $r_k$  and  $q_k$  for  $k_1 \leq k < i \leq n$ , we set

$$r_i = \min\{j \in \{1, \dots, m\} \mid \forall k < i : j \not\equiv r_k \pmod{q_k}\}.$$

There must exist one of the remaining primes  $\pi_j \in \{\pi_{k_1}, \dots, \pi_{2n-4}\} \setminus \{q_{k_1}, \dots, q_{i-1}\}$  with  $r_i \equiv q_j \pmod{\pi_j}$  because  $\{1, \dots, m\}$  is completely covered and  $m = \omega_2(n)$  is maximum. If there are several appropriate primes  $\pi_j$  to choose from, we set  $q_i = \pi_j$  for the smallest  $\pi_j$  possible. These  $r_i$  and  $q_i$  inductively selected as described above complete the wanted permutation and tuple.  $\square$

**Example 2.1.** We give an example for  $n = 6$ . The primes to be considered are 5, 7, 11, and 13. The result is  $\omega_2(n)=24$ .

The permutations

$$\pi_1 = 5, \pi_2 = 11, \pi_3 = 7, \pi_4 = 5, \pi_5 = 13, \pi_6 = 13, \pi_7 = 7, \pi_8 = 11, \text{ with } q_1 = 1, q_2 = 2, q_3 = 3, q_4 = 4, q_5 = 5, q_6 = 7, q_7 = 8, q_8 = 12,$$

and

$$q_1 = 7, q_2 = 11, q_3 = 7, q_4 = 5, q_5 = 13, q_6 = 5, q_7 = 13, q_8 = 11, \text{ with } r_1 = 1, r_2 = 2, r_3 = 3, r_4 = 4, r_5 = 5, r_6 = 6, r_7 = 7, r_8 = 12$$

are equivalent because

$$k_1 = 1, k_2 = 7 \text{ with } q_{k_1} \equiv q_{k_2} \pmod{\pi_{k_2}}, \text{ i.e. } 1 \equiv 8 \pmod{7}, \text{ and}$$

$$q_{k_1} = \pi_{k_2}, r_{k_1} = q_{k_1}.$$

The other required congruences are obvious when  $q_6 = \pi_1$  and  $q_7 = \pi_6$ .

The Reduced Permutation Algorithm 2 (RPA2) as depicted in pseudocode 3 makes use of proposition 2.1 and skips all permutations for which there exists an equivalent permutation with a smaller prime at a compatible position.

---

**Algorithm 3** Reduced Permutation Algorithm 2 (RPA2).

---

```
procedure REDUCED_PERMUTATION_2(arr,plist,clist,k,ind,pilist,qlist)
  for i=k to n-2 do
    if qlist[ind]  $\not\equiv$  0 (mod plist[i]) then
      if forall j<ind : qlist[j]  $\not\equiv$  qlist[ind] (mod plist[i]) or pilist[j]<plist[i]
      then
        arr1=arr; fill_array(arr1,qlist[ind],plist[i])
        pilist1=pilist; qlist1=qlist
        pilist1[ind]=plist[i]; ind1=ind+1; qlist1[ind1]=next_free_position(arr1)
        plist1=plist; clist1=clist
        if clist[i]=2 then
          clist1[i]=1
          k1=k
          reduced_permutation_2(arr1,plist1,clist1,k1,ind1,pilist1,qlist1)
        else
          if k<n-2 then
            interchange(plist1[k],plist1[i])
            interchange(clist1[k],clist1[i])
            k1=k+1
            reduced_permutation_2(arr1,plist1,clist1,k1,ind1,pilist1,qlist1)
          else count_array(arr1)
          end if
        end if
      end if
    end if
  end for
end procedure
arr=empty_array                                ▷ Sequence array
plist=[ $p_3, \dots, p_n$ ]                          ▷ Array of primes
clist=[2,...,2]                                ▷ Array of prime counters
k=1                                              ▷ Starting prime array index
ind=1                                           ▷ Starting index of permutation
pilist=empty_array                             ▷ List of prime permutation
qlist=empty_array                             ▷ List of first unlabelled positions
qlist[ind]=1                                  ▷ Starting sequence position
reduced_permutation_2(arr,plist,clist,k,ind,pilist,qlist)  ▷ Recursion
```

---

## 2.2 Bounding the remaining number of coprimes

The principles of the basic algorithms described above can only be reasonably utilised if the exclusion of many of the theoretically possible cases from the calculation can be conclusively substantiated. The Basic Sequential Algorithm 2 processes all potential combinations of residue classes. When particular combinations can be excluded from the analysis, the computational effort can be improved upon as is done in the Reduced Permutation Algorithm 2. A remainder combination may be discarded because it

actually cannot cover a sequence of the considered length. This decision must be based on proved criteria, which we derive in the following section.

The general idea was independently realised by Hagedorn [3] and Morack [6] in very similar approaches for the computation of Jacobsthal's original function. A modified version was applied to the paired Jacobsthal function [14] as well.

Euler's totient function  $\varphi(n)$  is known to be the number of positive integers up to a given integer  $n$  that are coprime to  $n$ . Costello and Watts used a specific generalisation of this function for the construction of a computational bound of Jacobsthal's function [1]. This generalisation counts the number of integers in a given sequence which are coprime to given primes. Following this basic idea, we are looking at the topic the other way round and consider pairs of integers in addition.

The function  $\psi_2(a, b, m, k)$  is the number of integer pairs in the paired progression  $\langle a, b \rangle_m$  which are not coprime to  $P_k = \prod_{i=3}^k p_i$ , i.e. which are divisible by one of the primes  $p_3, \dots, p_k$ . The index '2' stands for the domain of paired progressions. We emphasize that the first two primes  $p_1 = 2$  and  $p_2 = 3$  were omitted from the considerations. In other words,  $\psi_2(a, b, m, k)$  is the number of covered positions in the given integer sequence of length  $m$  where the set of remainders is condensed in  $a$  and  $b$ .

**Definition 2.1.** For  $a, b \in \mathbb{Z}$ ,  $m \in \mathbb{N}$ ,  $k \in \mathbb{N} \geq 3$ , we define

$$\begin{aligned}\psi_2(a, b, m, 1) &= \psi_2(a, b, m, 2) = 0, \\ \psi_2(a, b, m, k) &= |\{q \in \{1, \dots, m\} \mid \exists i \in \{3, \dots, k\} : \\ &\quad a + q \equiv 0 \pmod{p_i} \vee b + q \equiv 0 \pmod{p_i}\}|, \\ v_2(a, b, m, 1) &= v_2(a, b, m, 2) = 0, \text{ and} \\ v_2(a, b, m, k) &= \psi_2(a, b, m, k) - \psi_2(a, b, m, k-1).\end{aligned}$$

The difference  $v_2(a, b, m, k)$  corresponds to the number of integer pairs which are divisible by  $p_k$  but coprime to the primes  $p_3, \dots, p_{k-1}$ , i.e. the newly covered positions.

**Remark 2.1.** The sequence is completely covered if  $\psi_2(a, b, m, n) = m$ . The successive contribution of prime  $p_k$  is expressed by  $v_2(a, b, m, k)$ . Thus for  $3 \leq k \leq n$ , we get

$$\begin{aligned}\omega_2(n) &= \max \{m \in \mathbb{N} \mid \exists (a, b) \in \mathbb{Z}^2 : \\ \psi_2(a, b, m, n) &= \psi_2(a, b, m, k-1) + \sum_{i=k}^n v_2(a, b, m, i) = m\}.\end{aligned}$$

Let  $a, b$  solve the simultaneous congruences  $a \equiv -a_j \pmod{p_j}$  and  $b \equiv -b_j \pmod{p_j}$  for  $j = 3, \dots, n$ . Given a tentative length  $m$  of the sequence, the further processing of the corresponding set of remainders  $\{a_j, b_j\}$  can be skipped if

$$\sum_{i=k}^n v_2(a, b, m, i) < m - \psi_2(a, b, m, k-1)$$

can be proved for any  $k$ . Whereas  $\psi_2(a, b, m, k-1)$  can directly be counted, we below derive suitable upper bounds for  $\sum_{i=k}^n v_2(a, b, m, i)$  for an early and effective decision whether this inequality applies.

In a first step, we simplify our estimate and make it independent on specific progressions, i.e independent on  $a, b$ , or  $a_j, b_j$ , respectively. We consider the lowest possible number  $\psi_{2 \min}(m, k)$  of  $m$  consecutive integer pairs which are divisible by one of the primes  $p_3, \dots, p_k$ , and the highest possible number  $v_{2 \max}(m, k)$  of  $m$  consecutive integer pairs which are divisible by  $p_k$  but coprime to  $p_3, \dots, p_{k-1}$ .

**Definition 2.2.** Let  $m, k \in \mathbb{N}$ . Then

$$\psi_{2 \min}(m, k) = \min_{a, b \in \mathbb{Z}} \psi_2(a, b, m, k),$$

$$v_{2 \max}(m, k) = \max_{a, b \in \mathbb{Z}} v_2(a, b, m, k).$$

The term  $v_{2 \max}(m, k)$  can be bounded as the result of combinatorial considerations as follows.

**Lemma 2.2.** Let  $\lfloor x \rfloor$  denote the maximum integer not exceeding  $x \in \mathbb{R}$ ,  $m \in \mathbb{N}$ , and  $k \in \mathbb{N} \geq 3$ . Then

$$v_{2 \max}(m, k) \leq r_{m,k} - \psi_{2 \min}(r_{m,k}, k-1) + r_{m-1,k} - \psi_{2 \min}(r_{m-1,k}, k-1)$$

where  $r_{m,k} = 1 + \left\lfloor \frac{m-1}{p_k} \right\rfloor$ .

*Proof.* The number of multiples of  $p_k$  in a sequence of  $m$  consecutive integers is at most  $r_{m,k}$ . Every sequence contains at least  $r_{m,k} - 1$  such terms. The number of integer pairs in a paired progression of length  $m$  which are divisible by  $p_k$  is then at most  $r_{m,k} + r_{m-1,k}$  if the difference of pair elements is not a multiple of  $p_k$ . Otherwise, it would be not greater than  $2 \cdot r_{m,k} \geq r_{m,k} + r_{m-1,k}$ .

Let  $p_k \cdot (a + j)$  and  $p_k \cdot (b + j)$ ,  $a, b \in \mathbb{Z}$  and  $j = 1, \dots, r_{m,k}$ , be representations of  $r_{m,k}$  consecutive multiples of  $p_k$ , each. Every term  $p_k \cdot (a + j)$  or  $p_k \cdot (b + j)$  is divisible by  $p_i$  for  $i \in \{3, \dots, k-1\}$  if and only if  $p_i \mid (a + j)$  or  $p_i \mid (b + j)$ , respectively, because  $p_i \perp p_k$ .

$$p_i \mid (a + j) \Leftrightarrow p_i \mid p_k \cdot (a + j), \text{ and } p_i \mid (b + j) \Leftrightarrow p_i \mid p_k \cdot (b + j).$$

The paired progression  $\langle a, b \rangle_{r_{m,k}}$  contains multiples of  $p_i$  at the same positions  $j$  as at least one of the arithmetic progressions  $\{p_k \cdot (a + j)\}$  or  $\{p_k \cdot (b + j)\}$ . The number of elements in this paired progression which are divisible by any  $p_i$ ,  $i = 3, \dots, k-1$  is therefore  $\psi_2(a, b, r_{m,k}, k-1) \geq \psi_{2 \min}(r_{m,k}, k-1)$ .  $\square$

The term  $r_{m,k}$  can directly be calculated whereas the function  $\psi_{2 \min}(m, k)$  requires complex computations. For this purpose, we applied a brute force algorithm very similar to the Basic Sequential Algorithm 2.1. While BSA2 intends to maximise the number of covered positions in a given array, the computation of  $\psi_{2 \min}(m, k)$  needs to minimise it. We provide a table of function values of  $\psi_{2 \min}(m, k)$  for  $m \leq 1000$  and  $k \leq 8$  in an ancillary file.

The function  $\psi_{2 \min}(m, k)$  grows very slowly with increasing  $k$  while the time needed for it explodes. So, it must be sufficient to limit the maximum considered prime for practical application.



**Corollary 2.3.** Let  $a, b \in \mathbb{Z}$ ,  $m, n, t \in \mathbb{N}$ ,  $k \in \mathbb{N} \geq 3$ , and  $r_{m,i} = 1 + \left\lfloor \frac{m-1}{p_i} \right\rfloor$ ,  $i = k, \dots, n$ . For any  $t < k$ ,

$$\sum_{i=k}^n v_2(a, b, m, i) \leq \sum_{i=k}^n r_{m,i} - \sum_{i=k}^n \psi_{2 \min}(r_{m,i}, t) + \sum_{i=k}^n r_{m-1,i} - \sum_{i=k}^n \psi_{2 \min}(r_{m-1,i}, t).$$

*Proof.* According to lemma 2.2,

$v_2(a, b, m, i) \leq v_{2 \max}(m, i) \leq r_{m,i} - \psi_{2 \min}(r_{m,i}, i-1) + r_{m-1,i} - \psi_{2 \min}(r_{m-1,i}, i-1)$  holds for any  $i = k, \dots, n$ . The function  $\psi_{2 \min}(m, k)$  is monotonically increasing in  $k$  because the contribution of the respective next greater prime cannot be negative. So,  $\psi_{2 \min}(r_{m,i}, i-1) \geq \psi_{2 \min}(r_{m,i}, t)$  and  $\psi_{2 \min}(r_{m-1,i}, i-1) \geq \psi_{2 \min}(r_{m-1,i}, t)$  are consequences of  $t < k \leq i$ .  $\square$

With the help of this corollary, we can efficiently improve the naïve sequential algorithm. We recall that the further processing of the set of remainders  $\{a_j, b_j\}$  for a tentative sequence length  $m$  can be skipped if  $\sum_{i=k}^n v_2(a, b, m, i) < m - \psi_2(a, b, m, k-1)$  can be proved for any  $k$ . In this context, it is sufficient to verify the criterion

$$\sum_{i=k}^n r_{m,i} - \sum_{i=k}^n \psi_{2 \min}(r_{m,i}, t) + \sum_{i=k}^n r_{m-1,i} - \sum_{i=k}^n \psi_{2 \min}(r_{m-1,i}, t) < m - \psi_2(a, b, m, k-1) \quad (2.1)$$

for a suitable  $t < k$ .

This is the fundamental idea of the Discarding Sequential Algorithm 2 (DSA2) 4 to compute values of  $\omega_2(n)$ . Starting with a sufficiently long empty array and a tentative sequence length  $m$ , the parameter  $m$  is increased if a longer sequence was found.

It has shown to be more efficient if the first cycles, which employ only small primes, were processed without checking for the possibility of rejection. In later stages of the recursion, say from  $p_{k^*}$  on, the criterion can be applied. If the table of  $\psi_{2 \min}$  includes the corresponding values for  $t = k-1$  then they are preferred. Otherwise, the largest possible  $t$  must be used.

Another modification can slightly speed up the algorithm. The criterion 2.1 need not be compared for the entire length  $m$  of the considered sequence. It is sufficient to take the maximum length  $m^*$  of a subsequence into account which includes all uncovered positions. While counting  $\psi_2(a, b, m, k-1)$ , the appropriate  $m^*$  can simply be determined as well.

---

**Algorithm 4** Discarding Sequential Algorithm 2 (DSA2).

---

```
procedure DISCARDING_SEQUENTIAL_2(arr,k)
  for i=1 to plist[k]-2 do
    arr1=arr; fill_array(arr1,i,plist[k])
    for j=i+1 to plist[k]-1 do
      arr2=arr1; fill_array(arr2,j,plist[k])
      if k<n-2 then
        go_on=true
        if k ≥ k* then
          if criterion 2.1 fulfilled then go_on=false
          end if
        end if
        if go_on=true then discarding_sequential_2(arr2,k+1)
        end if
      else count_array(arr2)
        if longer_sequence_found then increase_m
        end if
      end if
    end for
  end for
end procedure
arr=empty_array                                ▷ Sequence array
m=starting_sequence_length                      ▷ Starting sequence length
plist=[p3,...,pn]                              ▷ Array of primes
k=1                                              ▷ Starting prime array index
k*=starting_index_for_criterion                 ▷ Starting prime array index for criterion
discarding_sequential_2(arr,k)                  ▷ Recursion
```

---

Although the DSA2 algorithm includes an efficient way to recognise inappropriate remainder combinations, it is time-consuming especially for large primes. The number of permutations to be considered in the RPA2 algorithm, however is much lower than the number of possible remainder combinations. The connection of these two principles in a Combined Reduced Permutation and Discarding Sequential Algorithm 2 (CRPDSA2) 5 can make the advantages of both ideas work together [15].

For smaller primes, the DSA2 algorithm is applied sequentially up to a fixed prime. The remaining primes are handled with the RPA2 algorithm which was extended by a test of an modified DSA2-criterion. The number of necessary cases can thus rigorously be reduced. An optimum point for the switch between both sub-algorithms was empirically found at  $p_n/2$  when  $p_n$  is the largest prime considered. We request  $p_{k^*} < p_n/2$ .

---

**Algorithm 5** Combined Reduced Permutation and  
Discarding Sequential Algorithm 2 (CRPDSA2).

---

```

procedure COMBINED_2(arr,plist,clist,k,ind,pilist,qlist)
  if  $p_k < p_k/2$  then ▷ DSA2 part
    for i=1 to plist[k]-2 do arr1=arr; fill_array(arr1,i,plist[k])
      for j=i+1 to plist[k]-1 do arr2=arr1; fill_array(arr2,j,plist[k]); go_on=true
      if  $k \geq k^*$  then
        if criterion 2.1 fulfilled then go_on=false end if
      end if
      if go_on=true then
        combined_2(arr2,plist,clist,k+1,ind,pilist,qlist)
      end if
    end for
  end for
  else
    if empty_qlist then ind=2*k-1; fill_qlist; fill_pilist end if
    for i=k to n-2 do ▷ RPA2 part
      if qlist[ind]  $\not\equiv 0 \pmod{\text{plist}[i]}$  then
        if forall j<ind : qlist[j]  $\not\equiv \text{qlist[ind]} \pmod{\text{plist}[i]}$  or  $\text{plist}[j] < \text{plist}[i]$ 
        then
          arr1=arr; fill_array(arr1,qlist[ind],plist[i]); plist1=plist; clist1=clist
          pilist1=pilist; qlist1=qlist; pilist1[ind]=plist[i]
          ind1=ind+1; qlist1[ind1]=next_free_position(arr1); go_on=true
          if modified criterion 2.1 fulfilled then go_on=false end if
          if go_on=true then
            if clist[i]=2 then
              clist1[i]=1
              k1=k
              combined_2(arr1,plist1,clist1,k1,ind1,pilist1,qlist1)
            else
              if k<n-2 then
                interchange(plist1[k],plist1[i])
                interchange(clist1[k],clist1[i])
                k1=k+1
                combined_2(arr1,plist1,clist1,k1,ind1,pilist1,qlist1)
              else count_array(arr1)
                if longer_sequence_found then increase_m end if
              end if
            end if
          end if
        end if
      end if
    end for
  end if
end procedure

```

|                                                |                                            |
|------------------------------------------------|--------------------------------------------|
| arr=empty_array                                | ▷ Sequence array                           |
| m=starting_sequence_length                     | ▷ Starting sequence length                 |
| plist=[ $p_3, \dots, p_n$ ]                    | ▷ Array of primes                          |
| clist=[2, ..., 2]                              | ▷ Array of prime counters                  |
| k=1                                            | ▷ Starting prime array index               |
| k*=starting_index_for_criterion                | ▷ Starting prime array index for criterion |
| ind=1                                          | ▷ Starting index of permutation            |
| pilist=empty_array                             | ▷ List of prime permutation                |
| qlist=empty_array                              | ▷ List of first unlabelled positions       |
| combined_2(arr,plist,clist,k,ind,pilist,qlist) | ▷ Recursion                                |

---

## 2.3 Counting the actually remaining number of coprimes

The last algorithmic suggestion of this paper, how to directly compute  $\omega_2(n)$ , is an improvement of the DSA2 algorithm 4. The actually remaining number of coprimes in the sequence is exactly counted for every pending prime instead of using a general, estimated bound for it. This is more time-consuming for a specific sequence under consideration. On the other hand, exact counts are often lower than the bounds. So, corresponding remainder constellations can be rejected much earlier. This compensates for the time effort spent for counting the exact frequencies.

We redefine some functions of the last subsection in a more general way. They are not restricted to require primes in their ascending order any more. In addition, primes are allowed to coexist twice. The idea of permutations plays a role again.

**Definition 2.3.** Let  $(\pi_1, \dots, \pi_{2n-4})$ ,  $n \in \mathbb{N} > 2$ , be an arbitrary but fixed permutation of  $\{p_3, \dots, p_n\}$  with twofold repetition, and  $Q$  an integer tuple  $(q_1, \dots, q_{2n-4})$ . For  $m, k \in \mathbb{N}$ , we define

$$\begin{aligned}\psi_2^*(Q, m, 0) &= 0, \\ \psi_2^*(Q, m, k) &= |\{q \in \{1, \dots, m\} \mid \exists i \in \{1, \dots, k\} : q \equiv q_i \pmod{\pi_i}\}|, \text{ and} \\ \nu_2^*(Q, m, k) &= \psi_2^*(Q, m, k) - \psi_2^*(Q, m, k-1).\end{aligned}$$

The difference  $\nu_2^*(Q, m, k)$  now corresponds to the number of integers covered by  $q_k \pmod{\pi_k}$  but not covered by  $q_i \pmod{\pi_i}$  for  $i \in \{1, \dots, k-1\}$  for  $k > 1$ . Again, let  $m$  be the tentative length of the sequence. The further processing of the corresponding permutation with the tuple  $Q$  can then be skipped if

$$\sum_{i=k}^{2n-4} \nu_2^*(Q, m, i) < m - \psi_2^*(Q, m, k-1)$$

can be proved for any  $k$ .

Every position in the sequence corresponds to a definite residue class for each prime. So, the number of remaining, non covered positions in the sequence which belong to a residue class can easily be counted. By this means, we derive individual bounds for  $\nu_2^*(Q, m, i)$  depending on the specific choice of  $Q$ .

**Definition 2.4.** Let  $(\pi_1, \dots, \pi_{2n-4})$ ,  $n \in \mathbb{N} > 2$ , be an arbitrary but fixed permutation of  $\{p_3, \dots, p_n\}$  with twofold repetition, and  $Q$  an integer tuple  $(q_1, \dots, q_{2n-4})$ . For  $m, k, t \in \mathbb{N}$  with  $k < t \leq 2 \cdot n - 4$ , we define

$$S_0 = \{1, \dots, m\},$$

$$S_k = \{q \in S_{k-1} \mid q \not\equiv q_k \pmod{\pi_k}\},$$

and for  $r_t \in \{1, \dots, \pi_t - 1\}$

$$\varrho(Q, m, k, t, r_t) = |\{q \in S_k \mid q \equiv r_t \pmod{\pi_t}\}|, \text{ and}$$

$$\varrho_{\max}(Q, m, k, t) = \max_{r_t \in \{1, \dots, \pi_t - 1\}} \varrho(Q, m, k, t, r_t).$$

The set of positions of a sequence  $\{1, \dots, m\}$  which are incongruent to  $q_i \pmod{\pi_i}$  for all  $i = 1, \dots, k$  is denoted by  $S_k$ , i.e. the set of so far uncovered positions. Given the set  $S_k$ ,  $\varrho(Q, m, k, k+1, r_{k+1})$  is the number of positions of the sequence which can be covered in the next step if  $q_{k+1} = r_{k+1}$  was chosen. We now relate the function  $\nu_2^*$  to  $\varrho_{\max}$ .

**Lemma 2.4.** Let  $(\pi_1, \dots, \pi_{2n-4})$ ,  $n \in \mathbb{N} > 2$ , be an arbitrary but fixed permutation of  $\{p_3, \dots, p_n\}$  with twofold repetition,  $Q$  an integer tuple  $(q_1, \dots, q_{2n-4})$ , and  $m, k, t \in \mathbb{N}$  with  $k < t \leq 2 \cdot n - 4$ . Then

$$\nu_2^*(Q, m, t) \leq \varrho_{\max}(Q, m, k, t).$$

*Proof.* By definition, there exists an  $r_t \in \{1, \dots, \pi_t - 1\}$  so that

$$\nu_2^*(Q, m, t) = \varrho(Q, m, t-1, t, r_t). \quad \text{For } k < t, \text{ we get}$$

$$\varrho(Q, m, t-1, t, r_t) \leq \varrho(Q, m, k, t, r_t) \leq \varrho_{\max}(Q, m, k, t) \text{ because } S_k \supseteq S_{t-1}. \quad \square$$

In consequence of lemma 2.4, it follows

$$\sum_{i=k}^{2n-4} \nu_2^*(Q, m, i) \leq \sum_{i=k}^{2n-4} \varrho_{\max}(Q, m, k-1, i),$$

because  $i \geq k$  and  $k < t$ , and we can now formulate the criterion

$$\sum_{i=k}^{2n-4} \varrho_{\max}(Q, m, k-1, i) < m - \psi_2^*(Q, m, k-1) \quad (2.2)$$

for the rejection of the further processing of the corresponding set of remainders  $Q$  for a tentative sequence length  $m$ .

The key idea of the effective realisation of this criterion in an algorithm is choosing the residue class with the maximum possible number of newly covered positions  $\max_{t \in \{k, \dots, 2n-4\}} \varrho_{\max}(Q, m, k-1, t)$  in every recursion cycle of level  $k$ . This choice implies a permutation algorithm because it selects  $\pi_t$  as the next prime. At the same time, it selects the residue class  $r_t \pmod{\pi_t}$  with  $\varrho(Q, m, k-1, t, r_t) = \max_{t \in \{k, \dots, 2n-4\}} \varrho_{\max}(Q, m, k-1, t)$ . Thus, the so-called Greedy Permutation Algorithm 2 (GPA2) 6 combines permutations with respect to primes and to remainders.

After level  $k + 1$  of recursion was done for that specific choice, the following cycles of level  $k$  do not need to consider the consumed  $r_t \bmod \pi_t$  again because all combinations of it were thereby examined. Otherwise, equivalent permutations would be considered. For the following cycles of level  $k$ , exclusively, the corresponding  $\varrho(Q, m, k - 1, t, r_t)$  is set to be 0, and  $\varrho_{\max}(Q, m, k - 1, t)$  is determined anew.

Because of the specific choice of the remainders  $r_t$ , the Greedy Permutation Algorithm (GPA2) is confined to process only prime permutations with  $\varrho(Q, m, i - 1, i, r_i) \leq \varrho(Q, m, j - 1, j, r_j)$  for  $i < j$ , i.e. the contribution of the primes is monotonically decreasing with the permutation order. Furthermore, a cyclic inner permutation of primes with the same contribution is prevented by blocking those  $r_t \bmod \pi_t$  always consumed at an earlier level.

It can be shown that the GPA2 algorithm is again more efficient if the first cycles, which employ only small primes, were processed simply sequentially without any checking for the possibility of rejection. This corresponds to the Basic Sequential Algorithm 2.1. In later stages of the recursion, say from  $p_{k^*}$  on, the new criterion will be applied, and the recursion changes to the true Greedy Permutation Algorithm.

---

**Algorithm 6** Greedy Permutation Algorithm 2 (GPA2).

---

```
procedure GREEDY_PERMUTATION_2(arr,k,ind,ftab)
  if k<k* then                                     ▷ Sequential part
    for i=1 to plist[k]-2 do arr1=arr; fill_array(arr1,i,plist[k])
      for j=i+1 to plist[k]-1 do arr2=arr1; fill_array(arr2,j,plist[k])
        greedy_permutation_2(arr2,k+1,ind,ftab)
      end for
    end for
  else
    if k=k* then ind=2*k+1
      fill_frequency_table_of_remainders(ftab)
    end if
    if ind<2*n-4 then                               ▷ Greedy permutation part
      update_q_max(...,t); go_on=true
      if criterion 2.2 fulfilled then go_on=false end if
      if go_on=true then                               ▷ Permutation level ind+1
        select_appropriate_r_t_and_pi_t; arr1=arr; fill_array(arr1,r_t,pi_t)
        ftab1=ftab; update_frequency_table_of_remainders(ftab1)
        greedy_permutation_2(arr1,k*+1,ind+1,ftab1)
      end if
      delete_frequency_of_r_t_mod_pi_t(ftab)
      if exists_non-zero_frequency_mod_pi_t(ftab) then ▷ Permutation level ind
        greedy_permutation_2(arr,k*+1,ind,ftab)
      end if
    else count_array(arr)
      if longer_sequence_found then increase_m end if
    end if
  end if
end procedure
arr=empty_array                                     ▷ Sequence array
m=starting_sequence_length                         ▷ Starting sequence length
plist=[p3,...,pn]                                   ▷ Array of primes
k=1                                                 ▷ Starting prime array index
k*=starting_index_for_criterion                   ▷ Starting prime array index for criterion
ind=1                                              ▷ Starting index of permutation
ftab=empty_table                                  ▷ Frequency table of remainders
greedy_permutation_2(arr,k,ind,ftab)              ▷ Recursion
```

---

## 2.4 Linear programming

There is another, direct way of computing  $\omega_2(n)$ . The problem of determining the maximum length of a sequence covered by a choice of residue classes according to proposition 1.5, statement (2), can be reformulated as a linear program. This idea was recently suggested by Resta [10]. It is not an algorithmic idea itself. But it is mathematically straightforward, simple, and ingenious. The possibility of just using standard software seems to be tempting. And in fact, this approach turned out to be very effective.

Resuming statement (2) of proposition 1.5, there exist two non-zero residue classes for every prime  $p_3, \dots, p_n$  so that every integer of the sequence  $\{1, \dots, m\}$  belongs to one of them.

$$\begin{aligned} &\exists a_i, b_i \in \{1, \dots, p_i - 1\}, i = 3, \dots, n : \\ &\forall q \in \{1, \dots, m\} \exists i \in \{3, \dots, n\} : q \equiv a_i \vee q \equiv b_i \pmod{p_i}. \end{aligned}$$

For every possible residue class, we define a binary variable  $x_{i,j} \in \{0, 1\}$ ,  $i \in \{3, \dots, n\}, j \in \{1, \dots, p_i - 1\}$  where  $x_{i,j} = 1$  if and only if  $j = a_i$  or  $j = b_i$ .

For the description of the sequence characterised as above, we formulate two sets of constraints. First, exactly two remainders should be chosen for each prime. Second, every position in the sequence  $\{1, \dots, m\}$  should be covered by at least one of the residue classes.

$$\begin{aligned} \sum_{j=1}^{p_i-1} x_{i,j} &= 2, \quad i = 3, \dots, n, \\ \sum_{\substack{i=3 \\ p_i \nmid q}}^n x_{i,q \bmod p_i} &\geq 1, \quad q = 1, \dots, m. \end{aligned} \tag{2.3}$$

The question of interest is whether or not there exist feasible solutions of these constraints. An objective function is not really needed. So, a dummy objective like

$$\max \sum_{i=3}^n \sum_{j=1}^{p_i-1} x_{i,j}$$

completes the integer linear program (ILP) with binary variables.

In order to calculate  $\omega_2(n)$ , a trial and error approach like nested intervals or the like might be applied, solving the described ILP for different  $m$ . If the system has any feasible solutions for  $m$  and none for  $m + 1$  then  $\omega_2(n) = m$ .

The search for the maximum suitable  $m$  can also be embedded into a single, extended ILP. Let  $m_1 < \omega_2(n)$  and  $m_2 > \omega_2(n)$  be tentative assumptions. We define additional binary variables  $y_k \in \{0, 1\}$ ,  $k \in \{m_1, \dots, m_2\}$  where  $y_k = 1$  if and only if position  $k$  in the sequence is covered by any of the residue classes under consideration, and formulate the following linear program with binary variables.



$$\begin{aligned}
& \max \quad \sum_{k=m_1}^{m_2} 2^{m_2-k} \cdot y_k, \\
& \sum_{j=1}^{p_i-1} x_{i,j} = 2, \quad i = 3, \dots, n, \\
& \sum_{\substack{i=3 \\ p_i \nmid q}}^n x_{i,q \bmod p_i} \geq 1, \quad q = 1, \dots, m_1 - 1, \\
& \sum_{\substack{i=3 \\ p_i \nmid k}}^n x_{i,k \bmod p_i} - y_k \geq 0, \quad k = m_1, \dots, m_2.
\end{aligned} \tag{2.4}$$

This linear program can be solved by using an established ILP solver. There are three kinds of solutions:

- (1)  $y_k = 0$  for all  $k = m_1, \dots, m_2$ .

The choice of  $m_1$  was too large,  $\omega_2(n) < m_1$ . Another try with a smaller  $m_1$  is needed.

- (2)  $y_k = 1$  for all  $k = m_1, \dots, m_2$ .

The choice of  $m_2$  was too small,  $\omega_2(n) \geq m_2$ . Another try with a larger  $m_2$  is needed.

- (3)  $y_k = 1$  for all  $k = m_1, \dots, m < m_2$ ,  $y_{m+1} = 0$ .

Then  $\omega_2(n) = m$ . An appropriate sequence of the length  $m$  can be derived from the solution for the variables  $x_{i,j}$ . A longer sequence with the required properties cannot exist because of the choice of the objective function. Each of its coefficients is larger than the sum of the following ones.

The above described way of calculating  $\omega_2(n)$  is denoted by 'ILP2' in the results section. It is very simple but its feasibility is limited.

The computation time for solving an ILP according to 2.3 or 2.4 grows much faster than the dimension of the problem. This dimension can significantly be reduced when the remainders of small primes were fixed. In a sequential approach, Morack solved all reduced problems like 2.3 for every possible remainder combination of the first small primes [7]. If a feasible solution was found in any case, the considered length  $m$  was increased for further ILPs until  $m + 1$  leads to an infeasible problem. For all subsequent remainder combination, the new length  $m$  was applied.

Given  $k^* \in \mathbb{N} > 3$ , and  $1 \leq a_x, b_x \in \mathbb{Z} < p_x$  for  $3 \leq x < k^*$ . Then we consider the reduced ILP

$$\begin{aligned}
& \max \sum_{i=k^*}^n \sum_{j=1}^{p_i-1} x_{i,j}, \\
& \sum_{j=1}^{p_i-1} x_{i,j} = 2, \quad i = k^*, \dots, n, \\
& \sum_{\substack{i=k^* \\ p_i \nmid q}}^n x_{i,q \bmod p_i} \geq 1, \quad q = 1, \dots, m, \text{ and} \\
& \quad q \not\equiv a_x \wedge q \not\equiv b_x \pmod{p_x}, \quad 3 \leq x < k^*.
\end{aligned} \tag{2.5}$$

The execution of the exhaustive computation of  $\omega_2(n)$  by decomposing the entire problem into many reduced ILPs is summarised in the Portioned ILP2 Algorithm (PILP2) 7. In a BSA2-like procedure, all relevant remainder combinations for primes less than  $p_{k^*}$  are passed through. For each of them, the reduced ILP 2.5 is solved, and the results are gathered.

---

**Algorithm 7** Portioned ILP2 Algorithm (PILP2).

---

```

procedure PORTIONED_ILP_2(arr,k)
  if k < k* then                                     ▷ Sequential part
    for i=1 to plist[k]-2 do arr1=arr; fill_array(arr1,i,plist[k])
      for j=i+1 to plist[k]-1 do arr2=arr1; fill_array(arr2,j,plist[k])
        portioned_ILP_2(arr2,k+1)
      end for
    end for
  else
    solve_reduced_ILP_2.5                               ▷ ILP part
    while exists_feasible_solution do
      record_solution
      increase_m; extend_arr; solve_reduced_ILP_2.5
    end while
  end if
end procedure
arr=empty_array                                         ▷ Sequence array
m=starting_sequence_length                             ▷ Starting sequence length
plist=[p3,...,pn]                                       ▷ Array of primes
k=1                                                     ▷ Starting prime array index
k*=starting_index_for_ILP                             ▷ Starting prime array index for solving ILP
portioned_ILP_2(arr,k)                                 ▷ Recursion

```

---

## 2.5 Parallel processing

All depicted explicit algorithms can be processed in parallel in a simple way. All of them are organised as treelike recursive procedures. Given a fixed recursion level  $k^*$ , the recurrent computation can be prepared in a first step by executing the recursive procedures until level  $k^*$ , only. All relevant parameters defining the next procedure call for level  $k^* + 1$  are written to a separate parameter file. Now in a second step, the subsequent subtrees or series of them, each starting at level  $k^* + 1$ , can be processed to their end on different cores, processors, or even on different computers. The last step summarises all individual results of these subprocesses, including all sequences of maximum length.

Parallel computation can be used most efficiently by a prior sorting of the subtrees of level  $k^* + 1$  by descending  $\psi_2(a, b, m, k)$ . This leads to an earlier recognition of longer sequences on average. The rapid enlargement of the respective array prevents from examining many too small sequences unnecessarily, and therefore speeds up the entire approach.

## 3 Results

The algorithms described in section 2 act very differently concerning its computational effort. We computed the entire values of the function  $h_2(n)$  with  $n \leq 21$  or  $p_n \leq 73$ , respectively. In these calculations, we used several algorithms each suitable regarding computation time. The equality of corresponding results served as an implicit verification of the correctness of the implementations. All computed values for  $3 \leq n \leq 21$  fulfil the conjectured bound  $h_2(n) < p_n^2 - p_n$  [17].

For every investigated  $n$ , we performed an exhaustive retrieval for all existing sequences of maximum length while searching for  $\omega_2(n)$ . As far as we know, this has not been done ever before. We provide this data in ancillary files.

### 3.1 Calculated data

All algorithms output values of the function  $\omega_2(n)$  according to definition 1.10 as their main result. In addition, every compatible sequence of the appropriate length  $\omega_2(n)$  was recorded. The values of  $h_2(n)$ , see definition 1.8, were deduced from  $\omega_2(n)$  by applying corollary 1.3.

An initial illustration of the results is outlined in figure 1. We graph the values of  $h_2(n)$  and the number of sequences of length  $\omega_2(n)$ . This number considerably varies in a non-obvious manner. The conjectured upper bound  $p_n^2 - p_n$  for  $h_2(n)$  [17] is plotted in addition in a dashed line.

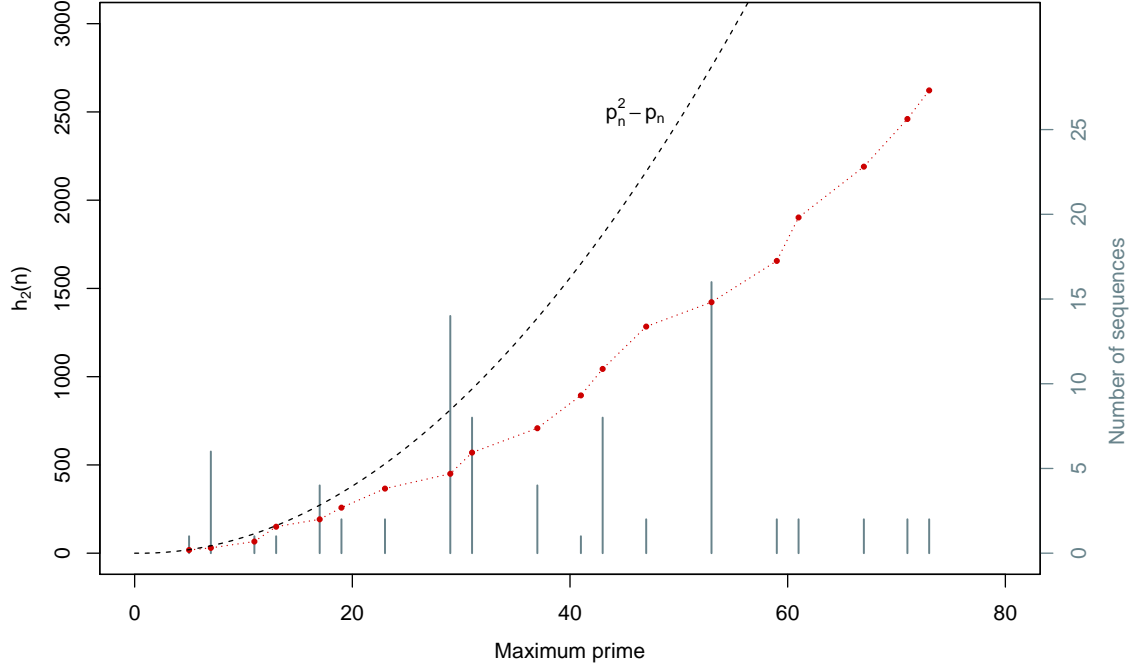

Figure 1: Values of the function  $h_2(n)$ , the conjectured bound  $p_n^2 - p_n$ , and the number of respective sequences of maximum length.

The complete data are provided in table 1 including the maximum processed prime  $p_n$ , the conjectured bound  $p_n^2 - p_n$ , the values of  $h_2(n)$  and  $\omega_2(n)$ , and the number of sequences  $n_{seq}$  for every  $n \leq 21$ .

| $n$ | $p_n$ | $p_n^2 - p_n$ | $h_2(n)$ | $\omega_2(n)$ | $n_{seq}$ |
|-----|-------|---------------|----------|---------------|-----------|
| 1   | 2     | 2             | 2        | —             | —         |
| 2   | 3     | 6             | 6        | —             | —         |
| 3   | 5     | 20            | 18       | 2             | 1         |
| 4   | 7     | 42            | 30       | 4             | 6         |
| 5   | 11    | 110           | 66       | 10            | 1         |
| 6   | 13    | 156           | 150      | 24            | 1         |
| 7   | 17    | 272           | 192      | 31            | 4         |
| 8   | 19    | 342           | 258      | 42            | 2         |
| 9   | 23    | 506           | 366      | 60            | 2         |
| 10  | 29    | 812           | 450      | 74            | 14        |
| 11  | 31    | 930           | 570      | 94            | 8         |

| $n$ | $p_n$ | $p_n^2 - p_n$ | $h_2(n)$ | $\omega_2(n)$ | $n_{seq}$ |
|-----|-------|---------------|----------|---------------|-----------|
| 12  | 37    | 1332          | 708      | 117           | 4         |
| 13  | 41    | 1640          | 894      | 148           | 1         |
| 14  | 43    | 1806          | 1044     | 173           | 8         |
| 15  | 47    | 2162          | 1284     | 213           | 2         |
| 16  | 53    | 2756          | 1422     | 236           | 16        |
| 17  | 59    | 3422          | 1656     | 275           | 2         |
| 18  | 61    | 3660          | 1902     | 316           | 2         |
| 19  | 67    | 4422          | 2190     | 364           | 2         |
| 20  | 71    | 4970          | 2460     | 409           | 2         |
| 21  | 73    | 5256          | 2622     | 436           | 2         |

Table 1: Computation results.

For every sequence of maximum length, there exists a reverse sequence according to corollary 1.6. Our results include a few self-symmetric sequences. All single sequences for  $n \in \{3, 5, 6, 13\}$  are self-symmetric by default. Two more self-symmetric sequences exist for  $n = 4$  with the permutations  $\{5, 7, 7, 5\}$  and  $\{7, 5, 5, 7\}$  according to remark 1.8, paragraph (3). No other sequences of maximum length with this property were found.

### 3.2 Computation time

All algorithms were implemented and executed on a common PC with an i7 processor at boosted 3.9 GHz. For solving the respective integer linear programs, we utilised SYMPHONY software [9, 5].

All algorithms except ILP2 were realised in a single thread application. For ILP2 solving the equations 2.4, however, we forced SYMPHONY to use all threads in parallel. The corresponding time needs were enlarged by an empirically estimated factor to make them comparable.

The time consumption of each algorithm rapidly grows with the number of primes. Figure 2 depicts this growth as well as the variation between different algorithms. A quasi-logarithmic time scale  $\log(1 + t)$  was applied where  $t$  was the exact time need rounded to full seconds.

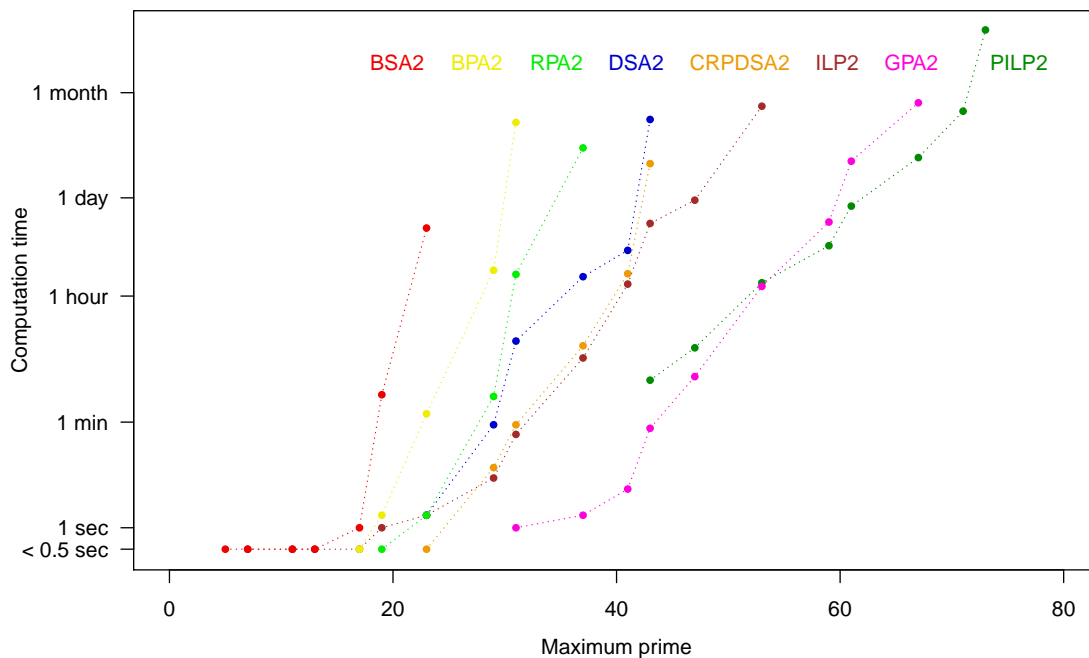

Figure 2: Comparison of the computational cost for various algorithms.

### 3.3 Ancillary data

In addition to this paper, we provide four files including the complete results of our calculations. The first file presents intrinsic data of the DSA2 algorithm 4.

#### **psi\_2\_min.txt**

This file contains a table of values of the function  $\psi_{2\min}(m, k)$  as described in definition 2.2 for  $m \leq 1000$  and  $k \leq 8$ . The data were computed using a brute force approach very similar to the Basic Sequential Algorithm 2 1. While BSA2 intends to maximise the number of covered positions in a given array, the computation of  $\psi_{2\min}(m, k)$  needs to minimise it.

The other ancillary files contain exhaustive lists of all sequences of the appropriate maximum lengths. According to proposition 1.5, these sequences can be represented in three ways as always has been concluded in remark 1.8.

#### **moduli\_2.txt**

This file contains the modulus-representation of the sequences. In remark 1.8, paragraph (1), every position  $q \in \{1, \dots, m\}$  of the sequence was related to at least one prime modulus  $p_i$ ,  $i \in \{3, \dots, n\}$ . The progression of primes  $p_q$ ,  $q \in \{1, \dots, m\}$  of the minimum appropriate moduli  $p_q$  each position  $q$  is a unique representation of the sequence under consideration.

#### **remainders\_2.txt**

This file contains the remainder-representation of the sequences, i.e. the ordered set of remainders  $a_i, b_i \pmod{p_i}$ ,  $i \in \{3, \dots, n\}$  as described in remark 1.8, paragraph (2).

#### **permutations\_2.txt**

This file contains the permutation-representation of the sequences, i.e. the permutation of primes  $\pi_i$ ,  $i \in \{1, \dots, 2n - 4\}$  as described in remark 1.8, paragraph (3).

The sequences in "remainders\_2.txt" are separately sorted for each  $n$  by ascending remainders. This order was maintained in the other files "permutations\_2.txt" and "moduli\_2.txt" to make a direct comparison possible.

### 3.4 Final remarks

All depicted algorithms may also be applied to arbitrary sets of different primes. The specific choice of consecutive primes was not necessarily required. With the help of prime separation as described in remark 1.6, all values of the paired Jacobsthal function  $j_2(n)$  can therefore be computed using a generalised implementation of one of these algorithms.

### Acknowledgement

The authors would like to express their appreciation to the On-Line Encyclopedia of Integer Sequences [8]. It provides an exceptional collection of integer progressions. This data is very informative and helps discover new items and links within the wide field of number theory.

Furthermore, the work of the COIN-OR project [5] is highly acknowledged. Modern approaches in computational operations research are developed, implemented, and disseminated in open source software.

### Contact

marioziller@arcor.de  
axelmorack@live.com

## References

- [1] Fintan Costello and Paul Watts, *A computational upper bound on Jacobsthal's function*, arXiv:1208.5342 [math.NT] (2012).
- [2] Paul Erdős, *On the Integers Relatively Prime to  $n$  and a Number-Theoretic Function Considered by Jacobsthal*, MATHEMATICA SCANDINAVICA **10** (1962), 163–170.
- [3] Thomas R. Hagedorn, *Computation of Jacobsthal's Function  $h(n)$  for  $n < 50$* , Mathematics of Computation **78** (2009), no. 266, 1073–1087.
- [4] Ernst Jacobsthal, *Über Sequenzen ganzer Zahlen, von denen keine zu  $n$  teilerfremd ist. I*, D.K.N.V.S. Forhandlinger **33** (1960), no. 24, 117–124.
- [5] Robin Lougee-Heimer, *The Common Optimization INterface for Operations Research: Promoting Open-source Software in the Operations Research Community*, IBM J. Res. Dev. **47** (2003), no. 1, 57–66.
- [6] John F. Morack, *Contribution to OEIS A072752 [11]*, private communication (2014), <http://oeis.org/A072752>.

- [7] John F. Morack, *Contribution to OEIS A072753 [12]*, private communication (2016), <http://oeis.org/A072753>.
- [8] OEIS Foundation Inc., *The On-Line Encyclopedia of Integer Sequences*, (2011), <http://oeis.org>.
- [9] Ted Ralphs, Menal Guzelsoy, Ashutosh Mahajan, and Laszlo Ladanyi, *SYMPHONY*, version 5.6.14 (2016), <https://projects.coin-or.org/SYMPHONY>.
- [10] Giovanni Resta, *Contribution to OEIS A072753 [12]*, private communication (2015), <http://oeis.org/A072753>.
- [11] Mario Ziller, *The On-Line Encyclopedia of Integer Sequences [8]*, Sequence A072752 (2002), <http://oeis.org/A072752>.
- [12] Mario Ziller, *The On-Line Encyclopedia of Integer Sequences [8]*, Sequence A072753 (2002), <http://oeis.org/A072753>.
- [13] Mario Ziller, *Contribution to OEIS A072753 [12]*, private communication (2005), <http://oeis.org/A072753>.
- [14] Mario Ziller, *Contribution to OEIS A072753 [12]*, private communication (2014), <http://oeis.org/A072753>.
- [15] Mario Ziller, *Contribution to OEIS A072753 [12]*, private communication (2015), <http://oeis.org/A072753>.
- [16] Mario Ziller and John F. Morack, *Algorithmic concepts for the computation of Jacobsthal's function*, arXiv:1611.03310 [math.NT] (2016).
- [17] Mario Ziller and John F. Morack, *Divisibility in paired progressions, Goldbach's conjecture, and the infinitude of prime pairs*, arXiv:1706.00317 [math.NT] (2017).
